# Supplementary material for: Ensuring Ground Truth Accuracy in Healthcare with the EVINCE framework
Source: arXiv:2405.15808 source file (2024-05-28)
Supplement: Supplementary file 1 [file AppendixAth.tex]

Yes, the diseases you mentioned—Arthritis, Cervical Spondylosis, Osteoarthritis, Polymyalgia Rheumatica, Fibromyalgia, and Lupus—are all related in that they are conditions affecting the musculoskeletal system and connective tissues, albeit in different ways. Here’s a brief overview of each and their interrelations:

Arthritis
Definition: A general term for conditions affecting the joints and surrounding tissues. It involves inflammation and can result in pain, stiffness, and swelling in the joints.
Types: Includes many types, such as rheumatoid arthritis (an autoimmune disease) and osteoarthritis (due to wear and tear).
Cervical Spondylosis
Definition: Also known as neck arthritis or cervical osteoarthritis, it is a condition involving changes to the bones, discs, and joints of the neck caused primarily by aging and wear and tear.
Symptoms: Neck pain and stiffness, which may extend to neurological symptoms if nerve compression occurs.
Osteoarthritis
Definition: The most common form of arthritis, caused by the breakdown of joint cartilage and underlying bone, usually due to age and wear and tear.
Symptoms: Pain, swelling, reduced motion in the affected joints.
Polymyalgia Rheumatica
Definition: An inflammatory disorder causing muscle pain and stiffness around the shoulders and hips.
Symptoms: Severe muscle aches and stiffness, particularly in the morning or after being inactive.
Fibromyalgia
Definition: A long-term condition that causes pain all over the body along with other symptoms.
Symptoms: Widespread pain, fatigue, sleep problems, memory issues, and mood changes.
Lupus
Definition: Systemic lupus erythematosus (SLE) is an autoimmune disease where the immune system attacks its own tissues, causing widespread inflammation and tissue damage in the affected organs.
Symptoms: Joint pain, rash, and fatigue, along with potential effects on organs such as the kidneys, heart, lungs, and brain.
Relationships and Differences:
Inflammatory Nature: Most of these conditions (except typically fibromyalgia and certain aspects of osteoarthritis) involve some level of inflammation.
Autoimmune Component: Lupus, rheumatoid arthritis, and to some extent, polymyalgia rheumatica, involve autoimmune mechanisms where the body’s immune system attacks its own cells.
Chronic Pain: All these conditions can lead to chronic pain, though the nature and source of the pain might vary—ranging from joint degeneration in osteoarthritis to widespread pain in fibromyalgia.
Systemic vs. Localized Effects: Lupus is systemic, affecting multiple organs and tissues throughout the body. In contrast, osteoarthritis and cervical spondylosis are more localized, affecting specific joints or areas of the body.
Understanding these diseases' relationships helps in approaching their management holistically, particularly in recognizing overlapping symptoms and choosing treatments that address the comprehensive needs of the patient.
