# Supplementary material for: Ensuring Ground Truth Accuracy in Healthcare with the EVINCE framework
Source: arXiv:2405.15808 source file (2024-05-28)
Supplement: Supplementary file 2 [file AppendixB-LLMParingTheory.tex]

\section*{Appendix B: Theory: Optimal Pairing of LLMs for Diagnostic Accuracy}

\textbf{Statement:} A pair of LLMs achieving the best diagnosis accuracy in terms of stability, accuracy, and robustness is a pair that 1) is equivalent in information quality, and 2) has one LLM with high information entropy and the other with low information entropy.

\textbf{Proof:}

1. {Equivalence in Information Quality:} \\
   Under the robust aggregation framework, coupling LLMs with equivalent competence ensures the sensitivity issues of additive regret are managed effectively \cite{Arieli2018,Guo2024algorithmic}. Equivalent competence implies that the LLMs have a similar underlying quality in their ability to process and generate information, which is crucial for effective collaboration.

2. {Entropy Balance:} \\
   According to information theory \cite{shannon1948}, when two communicating LLMs have different information entropies—one high and one low—regarding their prediction distribution on a symptom list, the overall prediction accuracy and robustness are optimized.
   
   \begin{itemize}[leftmargin=1.2em, topsep=.05em, parsep=.05em]
       \item \textit{High-High Entropy:} Both LLMs generate diverse hypotheses with high uncertainty, leading to low accuracy but high robustness due to extensive exploration.
       \item \textit{Low-Low Entropy:} Both LLMs generate precise but narrow hypotheses, leading to high accuracy but low robustness as the system may fail to adapt to unexpected inputs.
       \item \textit{High-Low Entropy:} The high-entropy LLM explores a wide range of possibilities, while the low-entropy LLM refines and narrows these possibilities. This balance leverages the strengths of both high entropy (diverse hypothesis generation) and low entropy (focused hypothesis refinement), optimizing both accuracy and robustness.
   \end{itemize}

3. {Empirical Validation:} \\
   Our empirical study in Section~\ref{sec:exp-case2} illustrates the practical application of this theory. The study demonstrates that pairs of LLMs with one high and one low in information entropy outperform pairs with matched entropies in terms of diagnosis accuracy, robustness, and stability.

Therefore, the optimal configuration for achieving the best diagnosis accuracy, stability, and robustness is to pair LLMs with equivalent information quality but differing information entropy, specifically one high and one low.

\begin{table}[ht!]
\centering
\begin{small}
\begin{tabular}{|l|c|c|c|}
\hline
\textbf{Metric} & \textbf{High-High Entropy} & \textbf{Low-Low Entropy} & \textbf{High-Low Entropy} \\ \hline
Accuracy & Low & High & High \\ \hline
Diversity of Solutions & Very High & Low & Moderate \\ \hline
Convergence & Low & High & Moderate \\ \hline
Robustness & High & Low & High \\ \hline
Efficiency & Low & High & Moderate \\ \hline
\end{tabular}
\end{small}
\vspace{.1in}
\caption{Comparison of three entropy-based parings}
\label{tab:LLMComparison}
\end{table}

%%%%%%%%%

There are several research works that support the theory that combining high and low entropy in prediction distributions can optimize accuracy and robustness. For example, a study on Coupled Variational Autoencoders (VAE) demonstrated that combining different levels of entropy in the model's latent space improves both accuracy and robustness by reducing divergence between distributions and increasing the likelihood of correct reconstructions, especially when dealing with corrupted data.

In the context of machine learning, balancing high-entropy (diverse, exploratory) and low-entropy (focused, confident) sources allows for a comprehensive approach that mitigates the risks of overfitting and underfitting, thereby enhancing overall performance. This approach is grounded in information theory principles, which suggest that diverse information sources (high entropy) combined with confident, precise predictions (low entropy) can lead to more robust and accurate outcomes.
