# Supplementary material for: Ensuring Ground Truth Accuracy in Healthcare with the EVINCE framework
Source: arXiv:2405.15808 source file (2024-05-28)
Supplement: Supplementary file 3 [file AppendixF.tex]

\section{Appendix: Influenza vs. Cold}

Influenza (commonly known as the flu) and pneumonia are both respiratory illnesses, but they are caused by different pathogens and can affect the body in distinct ways. Here are the key differences and similarities:

Similarities
Symptoms: Both can cause cough, fever, breathing difficulties, and fatigue. These overlapping symptoms can sometimes make it difficult to differentiate between the two without medical testing.
Complications: Both can lead to serious health complications, especially in vulnerable populations like the elderly, the very young, or those with pre-existing health conditions.
Differences
Causative Agents: Influenza is caused by the influenza viruses (types A and B being the most common). Pneumonia can be caused by bacteria, viruses (including influenza viruses), or fungi. The most common bacterial cause is Streptococcus pneumoniae.
Part of the Respiratory System Affected: Influenza primarily infects the upper respiratory tract (nose, throat) and sometimes the lungs, while pneumonia primarily affects the alveoli (air sacs) of the lungs, filling them with fluid or pus.
Vaccination and Prevention: Vaccines are available for both influenza and pneumococcal pneumonia (which protects against the bacterial type caused by Streptococcus pneumoniae). The flu vaccine is recommended annually, while pneumonia vaccines are generally recommended based on age and health conditions.
Treatment: Influenza treatments typically focus on relieving symptoms and sometimes antiviral drugs if diagnosed early. Pneumonia treatments vary significantly based on the cause (bacterial pneumonia is treated with antibiotics, for example), and may require hospitalization if severe.
Because influenza can lead to pneumonia as a complication, it's important to prevent or treat influenza early to reduce the risk of developing pneumonia.
