# Supplementary material for: Ensuring Ground Truth Accuracy in Healthcare with the EVINCE framework
Source: arXiv:2405.15808 source file (2024-05-28)
Supplement: Supplementary file 4 [file AppendixH.tex]

\section*{Appendix E: Lung ---}

Analyzing the symptoms listed and correlating them with Bronchial Asthma, Tuberculosis, and Pneumonia, here's how each set of symptoms may likely align with these diseases:

Bronchial Asthma
Relevant Symptoms: Fatigue, cough, breathlessness, mucoid sputum. Asthma often includes cough and breathlessness, and can sometimes involve fatigue due to the effort of breathing or poor sleep from nighttime symptoms.
Matching Entries: #61 (fatigue, cough, breathlessness, family history, mucoid sputum) could be indicative of asthma, particularly if there's a noted family history of asthma or other atopic conditions.

Tuberculosis
Relevant Symptoms: Cough, high fever, breathlessness, mucoid sputum. Tuberculosis typically presents with a persistent cough (often producing phlegm or mucoid sputum), fever, and breathlessness. These symptoms are chronic and generally persist for several weeks.
Matching Entries: #58 (fatigue, cough, high fever, breathlessness, family history, mucoid sputum) and #59 (cough, high fever, breathlessness, family history, mucoid sputum) are quite consistent with TB, particularly if 'family history' refers to a history of TB or exposure to it.

Pneumonia
Relevant Symptoms: Fatigue, cough, high fever, breathlessness, mucoid sputum. Pneumonia typically causes high fever, productive cough (often with discolored or mucoid sputum), breathlessness, and can lead to systemic symptoms like fatigue.
Matching Entries: #60 (fatigue, high fever, breathlessness, family history, mucoid sputum) and #63 (fatigue, cough, high fever, breathlessness, mucoid sputum) strongly align with pneumonia, showing a combination of respiratory and systemic symptoms typical of an acute infection.

Other Considerations
Entry #65 (headache, chest pain, dizziness, loss of balance, lack of concentration) does not specifically align with asthma, TB, or pneumonia, but suggests other neurological or cardiovascular issues that may need further evaluation for conditions like vertigo, cardiovascular disease, or possibly a neurological disorder.
These assessments are based on typical symptom presentations and should be followed up with medical evaluations for accurate diagnosis and appropriate treatment.

\subsection*{Claude vs. GPT-4 w/ Label Bronchitis}

Symptoms: chills, fatigue, cough, high fever, breathlessness, sweating, malaise, phlegm, chest pain,
fast heart rate, and rusty sputum.

\paragraph{Claude's Diagnoses and Justifications}

After conducting further research and analyzing the detailed symptom analysis provided by GPT-4, I have revised my predictions to align more closely with the available information. Here are the updated top 5 candidate diseases with adjusted probability values and reasoning:

1. Pneumonia (60\%)
   - Justification: The presence of rusty sputum is a strong indicator of bacterial pneumonia, as it suggests the presence of blood in the sputum due to lung inflammation. The combination of high fever, chills, cough, breathlessness, chest pain, phlegm, and fast heart rate strongly supports the diagnosis of pneumonia. Rusty sputum is less common in other respiratory diseases, making pneumonia the most likely diagnosis.

2. Acute Bronchitis (15\%)
   - Justification: Acute bronchitis shares several symptoms with pneumonia, such as cough, phlegm, chest pain, and breathlessness. However, the presence of rusty sputum and high fever is less typical in acute bronchitis compared to pneumonia. While a secondary bacterial infection in acute bronchitis can cause these symptoms, it is less likely than pneumonia based on the given information.

3. Tuberculosis (TB) (15\%)
   - Justification: Tuberculosis can present with chronic cough, high fever, night sweats, malaise, fatigue, chest pain, and occasionally rusty sputum. The chronic nature of TB and the presence of specific symptoms like rusty sputum make it a potential diagnosis. However, the absence of other characteristic symptoms, such as significant weight loss and prolonged duration of symptoms, makes TB less likely than pneumonia in this case.

4. COVID-19 (7\%)
   - Justification: COVID-19 can cause a wide range of symptoms, including high fever, fatigue, cough, breathlessness, chest pain, and malaise. However, the presence of rusty sputum is not a common feature of COVID-19, making it less likely than pneumonia and TB based on the provided symptoms.

5. Influenza (Flu) (3\%)
   - Justification: Influenza typically presents with high fever, chills, fatigue, cough, and malaise. While chest pain and a fast heart rate can occur in severe cases, rusty sputum is rare in influenza unless there is a secondary bacterial infection. The presence of rusty sputum and the lower frequency of other characteristic symptoms make influenza the least likely diagnosis among the listed options.

These revised predictions and justifications take into account the detailed symptom analysis and clinical correlations provided by GPT-4. The adjustments made are based on a more thorough understanding of the specific symptoms and their relative importance in each disease. However, it is crucial to emphasize that these predictions are based on the available information and should not replace a professional medical evaluation. A definitive diagnosis requires a comprehensive assessment by a healthcare provider, including physical examination and diagnostic tests.

\subsection*{GPT-4's Diagnoses and Justifications}

Pneumonia (60\%)

Justification: The presence of rusty sputum is a strong indicator of bacterial pneumonia, suggesting blood in the sputum due to lung inflammation. The combination of high fever, chills, cough, breathlessness, chest pain, phlegm, and fast heart rate strongly supports pneumonia. Rusty sputum is less common in other respiratory diseases, making pneumonia the most likely diagnosis.

Acute Bronchitis (15\%)

Justification: Acute bronchitis shares several symptoms with pneumonia, such as cough, phlegm, chest pain, and breathlessness. However, the presence of rusty sputum and high fever is less typical in acute bronchitis compared to pneumonia. While a secondary bacterial infection in acute bronchitis can cause these symptoms, it is less likely than pneumonia based on the given information.
Tuberculosis (TB) (15\%)

Justification: Tuberculosis can present with chronic cough, high fever, night sweats, malaise, fatigue, chest pain, and occasionally rusty sputum. The chronic nature of TB and the presence of specific symptoms like rusty sputum make it a potential diagnosis. However, the absence of other characteristic symptoms, such as significant weight loss and prolonged duration of symptoms, makes TB less likely than pneumonia in this case.
COVID-19 (7\%)

Justification: COVID-19 can cause a wide range of symptoms, including high fever, fatigue, cough, breathlessness, chest pain, and malaise. However, the presence of rusty sputum is not a common feature of COVID-19, making it less likely than pneumonia and TB based on the provided symptoms.
Influenza (Flu) (3\%)

Justification: Influenza typically presents with high fever, chills, fatigue, cough, and malaise. While chest pain and a fast heart rate can occur in severe cases, rusty sputum is rare in influenza unless there is a secondary bacterial infection. The presence of rusty sputum and the lower frequency of other characteristic symptoms make influenza the least likely diagnosis among the listed options.
Conclusion:
These adjusted predictions and justifications take into account the detailed symptom analysis and clinical correlations. Pneumonia remains the most likely diagnosis due to the presence of rusty sputum and other specific symptoms. Tuberculosis and acute bronchitis follow with equal probabilities, with COVID-19 and influenza being less probable. For an accurate diagnosis, a comprehensive evaluation by a healthcare professional, including physical examination and diagnostic tests, is essential.
