# Supplementary material for: Ensuring Ground Truth Accuracy in Healthcare with the EVINCE framework
Source: arXiv:2405.15808 source file (2024-05-28)
Supplement: Supplementary file 5 [file AppendixDengueChik.tex]

\section*{Appendix D: SocraHealth Debate: Dengue Fever vs. Chikungunya}

\input{CaseStudy2}
