# Supplementary material for: Ensuring Ground Truth Accuracy in Healthcare with the EVINCE framework
Source: arXiv:2405.15808 source file (2024-05-28)
Supplement: Supplementary file 6 [file AppendixS.tex]

\section{Appendix S: Skin --- Fungal Infection, Psoriasis, and Impetigo}

Key Differences
Nature of Cause: Fungal infections are caused by fungi, psoriasis is an autoimmune disorder, and impetigo is a bacterial infection.
Symptom Presentation: Psoriasis is generally more chronic and non-contagious with scaling and plaques, fungal infections often itch and affect the skin's integrity, and impetigo is acute, highly contagious, and features sores and crusts.
Treatment Approaches: Treatments for these conditions differ significantly due to their underlying causes; antifungals for fungal infections, immune system modulators for psoriasis, and antibiotics for impetigo.
While they share the commonality of affecting the skin, their differences in etiology, presentation, and management are significant. Accurate diagnosis is crucial to ensure appropriate treatment for each condition.
